# Supplementary material for: AQuA: Analytical Quality Assessment for Optimizing Video Analytics Systems
Source: arXiv:2101.09752 source file (2021-10-25)
Supplement: Supplementary file 1 [file appendix.tex]

\begin{figure*}
    \centering
    \begin{subfigure}[t]{0.162\textwidth}
        \centering
        \includegraphics[width=\textwidth]{figs/distorted_all/n02098413_10590_artifact_21.JPEG}
        %\caption{Original}
    \end{subfigure}
    \begin{subfigure}[t]{0.162\textwidth}
        \centering
        \includegraphics[width=\textwidth]{figs/distorted_all/n02098413_10590_artifact_26.JPEG}
        %\caption{Original}
    \end{subfigure}
    \begin{subfigure}[t]{0.162\textwidth}
        \centering
        \includegraphics[width=\textwidth]{figs/distorted_all/n02098413_10590_artifact_31.JPEG}
        %\caption{Original}
    \end{subfigure}
        \begin{subfigure}[t]{0.162\textwidth}
        \centering
        \includegraphics[width=\textwidth]{figs/distorted_all/n02098413_10590_artifact_36.JPEG}
        %\caption{Original}
    \end{subfigure}
        \begin{subfigure}[t]{0.162\textwidth}
        \centering
        \includegraphics[width=\textwidth]{figs/distorted_all/n02098413_10590_artifact_41.JPEG}
        %\caption{Original}
    \end{subfigure}
        \begin{subfigure}[t]{0.162\textwidth}
        \centering
        \includegraphics[width=\textwidth]{figs/distorted_all/n02098413_10590_artifact_49.JPEG}
        %\caption{Original}
    \end{subfigure}
    \caption{Compression Artifact [20,50]}
\end{figure*}

\begin{figure*}
    \centering
    \begin{subfigure}[t]{0.162\textwidth}
        \centering
        \includegraphics[width=\textwidth]{figs/distorted_all/n02098413_10590_bright_0.1.JPEG}
        %\caption{Original}
    \end{subfigure}
    \begin{subfigure}[t]{0.162\textwidth}
        \centering
        \includegraphics[width=\textwidth]{figs/distorted_all/n02098413_10590_bright_0.4.JPEG}
        %\caption{Original}
    \end{subfigure}
    \begin{subfigure}[t]{0.162\textwidth}
        \centering
        \includegraphics[width=\textwidth]{figs/distorted_all/n02098413_10590_bright_0.7.JPEG}
        %\caption{Original}
    \end{subfigure}
        \begin{subfigure}[t]{0.162\textwidth}
        \centering
        \includegraphics[width=\textwidth]{figs/distorted_all/n02098413_10590_bright_1.3.JPEG}
        %\caption{Original}
    \end{subfigure}
        \begin{subfigure}[t]{0.162\textwidth}
        \centering
        \includegraphics[width=\textwidth]{figs/distorted_all/n02098413_10590_bright_2.8.JPEG}
        %\caption{Original}
    \end{subfigure}
        \begin{subfigure}[t]{0.162\textwidth}
        \centering
        \includegraphics[width=\textwidth]{figs/distorted_all/n02098413_10590_bright_4.8.JPEG}
        %\caption{Original}
    \end{subfigure}
    \caption{Variation of Brightness [0.1, 50]}
\end{figure*}

\begin{figure*}
    \centering
    \begin{subfigure}[t]{0.162\textwidth}
        \centering
        \includegraphics[width=\textwidth]{figs/distorted_all/n02098413_10590_contrast_0.2.JPEG}
        %\caption{Original}
    \end{subfigure}
    \begin{subfigure}[t]{0.162\textwidth}
        \centering
        \includegraphics[width=\textwidth]{figs/distorted_all/n02098413_10590_contrast_0.6.JPEG}
        %\caption{Original}
    \end{subfigure}
    \begin{subfigure}[t]{0.162\textwidth}
        \centering
        \includegraphics[width=\textwidth]{figs/distorted_all/n02098413_10590_contrast_0.9.JPEG}
        %\caption{Original}
    \end{subfigure}
        \begin{subfigure}[t]{0.162\textwidth}
        \centering
        \includegraphics[width=\textwidth]{figs/distorted_all/n02098413_10590_contrast_1.2.JPEG}
        %\caption{Original}
    \end{subfigure}
        \begin{subfigure}[t]{0.162\textwidth}
        \centering
        \includegraphics[width=\textwidth]{figs/distorted_all/n02098413_10590_contrast_2.3.JPEG}
        %\caption{Original}
    \end{subfigure}
        \begin{subfigure}[t]{0.162\textwidth}
        \centering
        \includegraphics[width=\textwidth]{figs/distorted_all/n02098413_10590_contrast_3.2.JPEG}
        %\caption{Original}
    \end{subfigure}
    \caption{Variation of Contrast [0.1, 50]}
\end{figure*}

\begin{figure*}
    \centering
    \begin{subfigure}[t]{0.162\textwidth}
        \centering
        \includegraphics[width=\textwidth]{figs/distorted_all/n02098413_10590_sp_0.05.JPEG}
        %\caption{Original}
    \end{subfigure}
    \begin{subfigure}[t]{0.162\textwidth}
        \centering
        \includegraphics[width=\textwidth]{figs/distorted_all/n02098413_10590_sp_0.11.JPEG}
        %\caption{Original}
    \end{subfigure}
    \begin{subfigure}[t]{0.162\textwidth}
        \centering
        \includegraphics[width=\textwidth]{figs/distorted_all/n02098413_10590_sp_0.19.JPEG}
        %\caption{Original}
    \end{subfigure}
        \begin{subfigure}[t]{0.162\textwidth}
        \centering
        \includegraphics[width=\textwidth]{figs/distorted_all/n02098413_10590_sp_0.28.JPEG}
        %\caption{Original}
    \end{subfigure}
        \begin{subfigure}[t]{0.162\textwidth}
        \centering
        \includegraphics[width=\textwidth]{figs/distorted_all/n02098413_10590_sp_0.34.JPEG}
        %\caption{Original}
    \end{subfigure}
        \begin{subfigure}[t]{0.162\textwidth}
        \centering
        \includegraphics[width=\textwidth]{figs/distorted_all/n02098413_10590_sp_0.48.JPEG}
        %\caption{Original}
    \end{subfigure}
    \caption{Low-light Noise [1, 100]}
\end{figure*}

\begin{figure*}
    \centering
    \begin{subfigure}[t]{0.162\textwidth}
        \centering
        \includegraphics[width=\textwidth]{figs/distorted_all/n02098413_10590_focal_1.JPEG}
        %\caption{Original}
    \end{subfigure}
    \begin{subfigure}[t]{0.162\textwidth}
        \centering
        \includegraphics[width=\textwidth]{figs/distorted_all/n02098413_10590_focal_5.JPEG}
        %\caption{Original}
    \end{subfigure}
    \begin{subfigure}[t]{0.162\textwidth}
        \centering
        \includegraphics[width=\textwidth]{figs/distorted_all/n02098413_10590_focal_9.JPEG}
        %\caption{Original}
    \end{subfigure}
        \begin{subfigure}[t]{0.162\textwidth}
        \centering
        \includegraphics[width=\textwidth]{figs/distorted_all/n02098413_10590_focal_12.JPEG}
        %\caption{Original}
    \end{subfigure}
        \begin{subfigure}[t]{0.162\textwidth}
        \centering
        \includegraphics[width=\textwidth]{figs/distorted_all/n02098413_10590_focal_15.JPEG}
        %\caption{Original}
    \end{subfigure}
        \begin{subfigure}[t]{0.162\textwidth}
        \centering
        \includegraphics[width=\textwidth]{figs/distorted_all/n02098413_10590_focal_19.JPEG}
        %\caption{Original}
    \end{subfigure}
    \caption{De-focus Blur [1, 20]}
\end{figure*}

\begin{figure*}
    \centering
    \begin{subfigure}[t]{0.162\textwidth}
        \centering
        \includegraphics[width=\textwidth]{figs/distorted_all/n02098413_10590_motion_5.JPEG}
        %\caption{Original}
    \end{subfigure}
    \begin{subfigure}[t]{0.162\textwidth}
        \centering
        \includegraphics[width=\textwidth]{figs/distorted_all/n02098413_10590_motion_9.JPEG}
        %\caption{Original}
    \end{subfigure}
    \begin{subfigure}[t]{0.162\textwidth}
        \centering
        \includegraphics[width=\textwidth]{figs/distorted_all/n02098413_10590_motion_15.JPEG}
        %\caption{Original}
    \end{subfigure}
        \begin{subfigure}[t]{0.162\textwidth}
        \centering
        \includegraphics[width=\textwidth]{figs/distorted_all/n02098413_10590_motion_20.JPEG}
        %\caption{Original}
    \end{subfigure}
        \begin{subfigure}[t]{0.162\textwidth}
        \centering
        \includegraphics[width=\textwidth]{figs/distorted_all/n02098413_10590_motion_24.JPEG}
        %\caption{Original}
    \end{subfigure}
        \begin{subfigure}[t]{0.162\textwidth}
        \centering
        \includegraphics[width=\textwidth]{figs/distorted_all/n02098413_10590_motion_28.JPEG}
        %\caption{Original}
    \end{subfigure}
    \caption{Distortion caused by Camera/Object Motion [5, 30]}
\end{figure*}

\begin{figure*}
    \centering
    \begin{subfigure}[t]{0.162\textwidth}
        \centering
        \includegraphics[width=\textwidth]{figs/distorted_all/n02098413_10590_gauss_22.JPEG}
        %\caption{Original}
    \end{subfigure}
    \begin{subfigure}[t]{0.162\textwidth}
        \centering
        \includegraphics[width=\textwidth]{figs/distorted_all/n02098413_10590_gauss_33.JPEG}
        %\caption{Original}
    \end{subfigure}
    \begin{subfigure}[t]{0.162\textwidth}
        \centering
        \includegraphics[width=\textwidth]{figs/distorted_all/n02098413_10590_gauss_54.JPEG}
        %\caption{Original}
    \end{subfigure}
        \begin{subfigure}[t]{0.162\textwidth}
        \centering
        \includegraphics[width=\textwidth]{figs/distorted_all/n02098413_10590_gauss_69.JPEG}
        %\caption{Original}
    \end{subfigure}
        \begin{subfigure}[t]{0.162\textwidth}
        \centering
        \includegraphics[width=\textwidth]{figs/distorted_all/n02098413_10590_gauss_81.JPEG}
        %\caption{Original}
    \end{subfigure}
        \begin{subfigure}[t]{0.162\textwidth}
        \centering
        \includegraphics[width=\textwidth]{figs/distorted_all/n02098413_10590_gauss_97.JPEG}
        %\caption{Original}
    \end{subfigure}
    \caption{Gaussian Noise [0.05, 0.5]}
\end{figure*}
